# Supplementary material for: SpatialMem: Metric-Aligned Long-Horizon Video Memory for Language Grounding and QA
Source: arXiv:2601.14895 source file (2026-10-23)
Supplement: Supplementary file 1 [file X_suppl.tex]

\clearpage
\setcounter{page}{1}
\maketitlesupplementary

\section{Pipeline Visualizations}
\label{sec:supp-pipeline}

Figure~\ref{fig:supp_pipeline} provides a high-resolution overview of the full SpatialMem pipeline.
It visualizes the stages from egocentric RGB input to a queryable 3D memory tree:

% \begin{itemize}
%   \item \textbf{RGB ingestion}: egocentric frames are sampled and normalized.
%   \item \textbf{Geometry estimation}: monocular pose+depth prediction produces a dense point cloud.
%   \item \textbf{Metric alignment}: floor-plane detection and rotation align the scene to an upright metric frame.
%   \item \textbf{Anchor construction}: walls, doors, and windows are detected as stable 3D planes/boxes and merged across views.
%   \item \textbf{Object lifting}: open-vocabulary 2D detections and masks are lifted to 3D boxes via back-projection.
%   \item \textbf{Memory tree}: a three-level tree organizes anchors (Level~1), objects (Level~2), and text descriptions (Level~3).
%   \item \textbf{Query execution}: language queries traverse the tree using geometric predicates (distance, orientation, visibility).
% \end{itemize}

\begin{figure*}[!t]
    \centering
    \includegraphics[width=\linewidth]{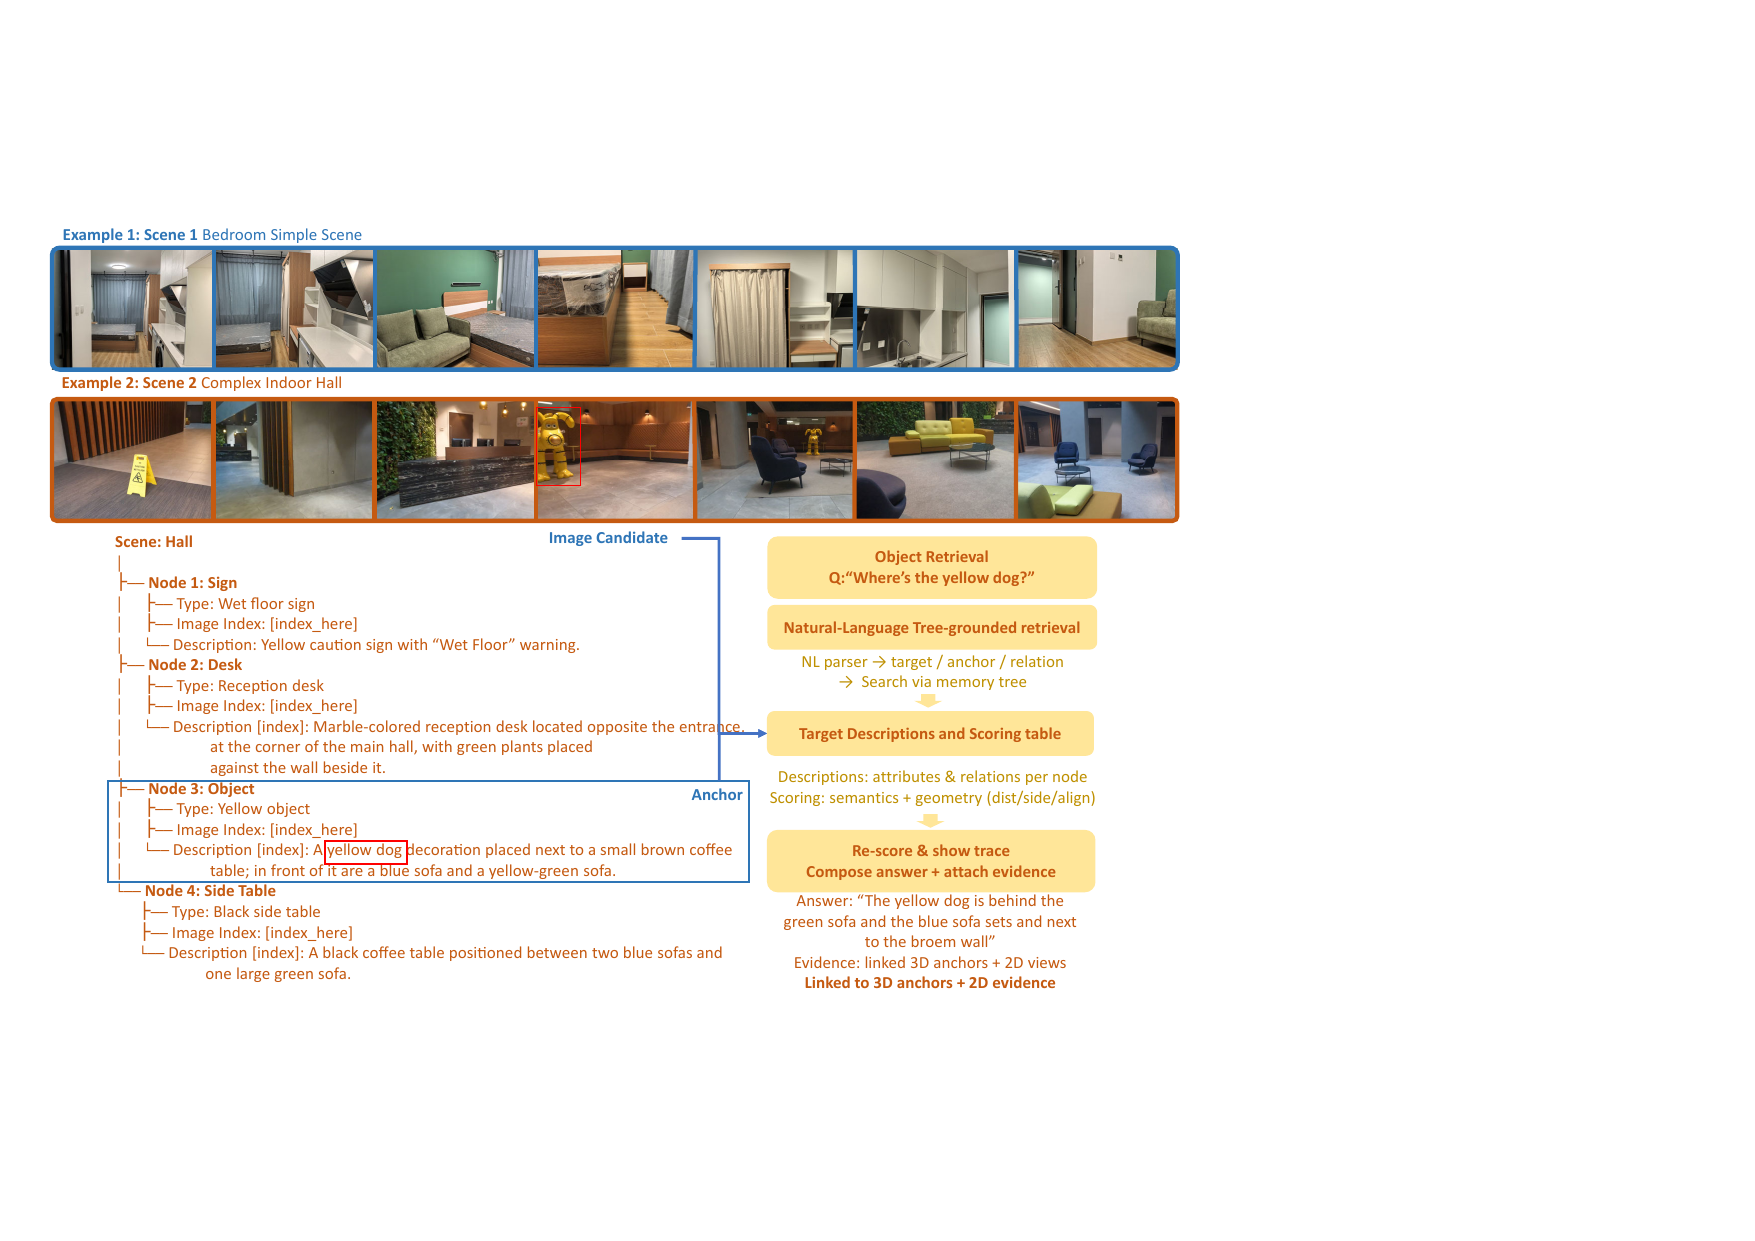}
    \caption{High-level SpatialMem pipeline. From left to right: egocentric RGB input,
    geometry and metric alignment, anchor and object construction, memory tree, and
    query execution via geometric and semantic reasoning.}
    \label{fig:supp_pipeline}
\end{figure*}

\begin{table*}[t]
  \centering
  \caption{Model size (per scene) and average testing time (seconds) across all models and tasks.}
  \label{size_and_time}
  \scriptsize
  \begin{tabular}{llcccccc}
    \toprule
    \textbf{model name} & \textbf{task name} &
    \textbf{memory size S1} & \textbf{memory size S2} & \textbf{memory size S3} &
    \textbf{avg time S1 (s)} & \textbf{avg time S2 (s)} & \textbf{avg time S3 (s)} \\
    \midrule
    navigation 3d & navigation & 2.3G & 3.4G & 5.1G & 7.3530 & 13.0530 & 16.0530 \\
    navigation 3d & object retrieval & 2.3G & 3.4G & 5.1G & 4.4220 & 10.1220 & 13.1220 \\
    gemini & navigation & online & online & online & 19.5833 & 25.2833 & 28.2833 \\
    gemini & object retrieval & online & online & online & 18.7226 & 24.4226 & 27.4226 \\
    llava & navigation & 13.72 GB & 13.72 GB & 13.72 GB & 22.0730 & 27.7730 & 30.7730 \\
    llava & object retrieval & 13.72 GB & 13.72 GB & 13.72 GB & 18.9901 & 22.9901 & 25.7062 \\
    openai 4.1 mini & navigation & online & online & online & 17.0989 & 20.9658 & 23.2326 \\
    openai 4.1 mini & object retrieval & online & online & online & 16.3337 & 19.3337 & 22.4849 \\
    Qwen 2.5 & navigation & online & online & online & 14.7300 & 16.7700 & 19.2600 \\
    Qwen 2.5 & object retrieval & online & online & online & 19.1000 & 22.1000 & 25.1700 \\
    Qwen local & navigation & 15.45 GB & 15.45 GB & 15.45 GB & 39.7447 & 42.7447 & 44.7447 \\
    Qwen local & object retrieval & 15.45 GB & 15.45 GB & 15.45 GB & 36.7896 & 38.7896 & 41.7896 \\
    InternVL local & navigation & 15.04 GB & 15.04 GB & 15.04 GB & 29.0453 & 32.0453 & 35.0453 \\
    InternVL local & object retrieval & 15.04 GB & 15.04 GB & 15.04 GB & 24.4894 & 27.4894 & 30.4894 \\
    miniCPM local & navigation & 16.20 GB & 16.20 GB & 16.20 GB & 26.1561 & 29.1561 & 32.1561 \\
    miniCPM local & object retrieval & 16.20 GB & 16.20 GB & 16.20 GB & 21.9345 & 24.9345 & 27.9345 \\
    \bottomrule
  \end{tabular}
\end{table*}

\section{Dataset and Capture Details}
\label{sec:supp-dataset}

We summarize the capture setup and the three egocentric indoor scenes used in our experiments. All information is taken directly from the project documentation.

\subsection*{Capture Setup}

\begin{itemize}
  \item \textbf{Camera device:}
    \begin{itemize}
      \item Lightweight pin-style \emph{LUCI} camera, worn for hands-free egocentric recording.
      \item Compact form factor suitable for continuous indoor navigation.
    \end{itemize}

  \item \textbf{Capture protocol:}
    \begin{itemize}
      \item Natural egocentric walk-throughs with forward-facing motion.
      \item Single continuous pass per scene; indoor-only; no additional constraints specified.
    \end{itemize}
\end{itemize}

\subsection*{Scene Characteristics}

\begin{itemize}
  \item \textbf{Scene~1 (Simple room):}
    \begin{itemize}
      \item Approx.\ \textbf{20\,m\textsuperscript{2}} indoor room.
      \item \textbf{30-minute} egocentric video.
      \item Standard furniture; clutter level not specified.
    \end{itemize}

  \item \textbf{Scene~2 (Suite main room / Entry hall):}
    \begin{itemize}
      \item Approx.\ \textbf{40\,m\textsuperscript{2}} entrance hall.
      \item \textbf{50-minute} continuous recording.
      \item Open layout; no further object details documented.
    \end{itemize}

  \item \textbf{Scene~3 (Laboratory / Storage):}
    \begin{itemize}
      \item Approx.\ \textbf{40\,m\textsuperscript{2}} laboratory storage area with higher spatial complexity.
      \item \textbf{60-minute} egocentric recording.
      \item Complex layout; detailed clutter description not provided.
    \end{itemize}
\end{itemize}

\section{Expanded Metrics and Error Analysis}
\label{sec:supp-metrics}

This section expands the metric definitions from previous experiment setup section of the main paper, providing full formulas and operational details for reproducibility.

\subsection{Notation}

Let $\mathcal{D}$ be the set of episodes.
For episode $i\in\mathcal{D}$, denote the goal location by $g_i$, the final user location by $\hat g_i$, the shortest path length by $L_i^\star$, and the executed path length by $L_i$.
Let $\mathbf{1}[\cdot]$ be the indicator function.
For navigation, we use:
a success distance threshold $d_{\mathrm{thr}}$ (e.g., $1\,\mathrm{m}$), proximity thresholds $\tau_{\text{near}},\tau_{\text{attach}}$, and an angular tolerance $\theta_{\text{rel}}$ for left/right/front/back judgments.
We report means over scenes with $95\%$ bootstrap confidence intervals.

\subsection{Task 1: Basic Relative Position Evaluation}
\label{sec:supp-rel-metrics}

This task evaluates whether the memory recovers basic spatial relations between entities
\[
\mathrm{rel} \in \{\text{left},\text{right},\text{front},\text{behind},\text{near},\text{on}\}.
\]
Each query specifies two targets, and the system returns an answer of the form
“$A$ is $\mathrm{rel}$ of $B$.”

Let $\mathcal{Q}$ be the set of queries, with predicted relation $\widehat{\mathrm{rel}}_q$ and ground-truth relation $\mathrm{rel}^\star_q$.
The main metric is the \emph{Relation Accuracy}:
\begin{equation}
\mathrm{Acc}_{\text{rel}}
\;=\;
\frac{1}{|\mathcal{Q}|}
\sum_{q\in\mathcal{Q}}
\mathbf{1}\!\left[
\, \widehat{\mathrm{rel}}_{q} = \mathrm{rel}^\star_{q} \,
\right].
\end{equation}

We also report anchor-specific accuracies.
For each Level-1 structural anchor $s$ (e.g., a particular wall, door, or window), we compute
$\mathrm{Acc}_{\text{rel}}(s)$ using only queries that reference $s$, and report a macro-average over anchors:
\begin{equation}
\mathrm{Acc}_{\text{rel}}^{\text{macro}}
\;=\;
\frac{1}{|\mathcal{S}|}
\sum_{s\in\mathcal{S}}
\mathrm{Acc}_{\text{rel}}(s).
\end{equation}

\subsubsection*{Operational definitions (relative relations)}

Left/right/front/behind are computed in the allocentric, upright frame.
Given a structural anchor with outward normal and a target object box, we classify the side relation using the signed angle between the anchor’s reference direction and the vector from the anchor to the object; predictions within $\theta_{\text{rel}}$ of the annotated side are counted as correct.

For predicates \texttt{near}/\texttt{attached}, let $B_o$ be the 3D box of object $o$ and $(\pi_e, B_e)$ be the plane/box of anchor $e$.
We use:
\begin{itemize}
  \item \texttt{attached} if
  $\min_{x\in B_o} \operatorname{dist}(x,\pi_e) < \tau_{\text{attach}}$,
  \item \texttt{near} if
  $\min_{x\in B_o} \operatorname{dist}(x,B_e) < \tau_{\text{near}}$,
\end{itemize}
with thresholds chosen empirically and shared across scenes.
Ambiguous boundary cases are lightly audited and excluded when necessary.

\subsection{Task 2: Navigation Metrics}
\label{sec:supp-nav-metrics}

We decompose navigation performance into (i) success rate, (ii) step-weighted completion, (iii) path efficiency, and (iv) error.

\subsubsection*{Navigation success rate}

An episode is successful if the final predicted goal lies within distance $d_{\mathrm{thr}}$ of the true target:
\begin{equation}
S_i^{\text{nav}}
=
\mathbf{1}\!\left[
\bigl\lVert \hat{g}_i - g_i \bigr\rVert_2
\le
d_{\mathrm{thr}}
\right].
\end{equation}
The navigation success rate is
\begin{equation}
\mathrm{SR}_{\text{nav}}
=
\frac{1}{|\mathcal{D}|}
\sum_{i\in\mathcal{D}}
S_i^{\text{nav}} \, .
\end{equation}

\subsubsection*{Step-weighted navigation completion}

Let each navigation description comprise $T_i$ ordered steps, with completion score $c_{i,t}\in[0,1]$ and non-negative weights $w_{i,t}$ (later steps can be up-weighted).
The per-episode completion is
\begin{equation}
\mathrm{StepComp}_i
=
\frac{\sum_{t=1}^{T_i} w_{i,t}\, c_{i,t}}{\sum_{t=1}^{T_i} w_{i,t}},
\end{equation}
and we report the average
\begin{equation}
\overline{\mathrm{StepComp}}
=
\frac{1}{|\mathcal{D}|}
\sum_{i\in\mathcal{D}}
\mathrm{StepComp}_i .
\end{equation}

\paragraph*{Operational definition (step completion).}
For textual steps, $c_{i,t}=1$ if the step’s verifiable condition (landmark reached/visible, turn executed) is satisfied by logs and geometry; graded values in $(0,1)$ are used when only partially satisfied (e.g., landmark reached but extra detour taken).

\subsubsection*{Path efficiency (SPL)}

We use the standard Success-weighted by Path Length (SPL):
\begin{equation}
\mathrm{SPL}
=
\frac{1}{|\mathcal{D}|}
\sum_{i\in\mathcal{D}}
S_i^{\text{nav}}
\cdot
\frac{L_i^\star}{\max(L_i,\, L_i^\star)} \, ,
\end{equation}
where $L_i^\star$ is the shortest-path length to the goal and $L_i$ is the executed path length.

\subsubsection*{Navigation error (NE)}

Navigation error is the mean final distance to the goal over failed episodes:
\begin{equation}
\mathrm{NE}
=
\frac{1}
{\left|\{\, i \in \mathcal{D} : S_i^{\text{nav}}=0 \,\}\right|}
\sum_{i \in \mathcal{D} : S_i^{\text{nav}}=0}
\bigl\lVert \hat{g}_i - g_i \bigr\rVert_2 .
\end{equation}
Distance thresholds, angular tolerances, and tie-breaking rules (e.g., for multiple near-optimal paths) are specified to match the main text.

\subsection{Task 3: Object Retrieval Metrics}
\label{sec:supp-obj-metrics}

Object retrieval episodes require locating a target object $o_i$ and confirming it (e.g., by description or pointer).

\subsubsection*{Retrieval success}

Let
\[
R_i
=
\mathbf{1}\!\left[\text{correct object $o_i$ confirmed}\right].
\]
The object retrieval success rate is
\begin{equation}
\mathrm{SR}_{\text{obj}}
=
\frac{1}{|\mathcal{D}|}
\sum_{i\in\mathcal{D}} R_i \, .
\end{equation}
When retrieval depends on navigation, an episode counts as fully successful only if both the goal is reached and the object is confirmed; we also report the two components separately in the main tables.

\subsubsection*{Hierarchical (tree) retrieval accuracy}

Each retrieved object node $\hat{v}_i$ has a parent chain from the root to $\operatorname{parent}(\hat{v}_i)$.
Let $v_i$ be the ground-truth node.

\emph{Parent accuracy} measures whether the immediate parent (e.g., container, room, or anchor) is correct:
\begin{equation}
\mathrm{Acc}_{\text{parent}}
=
\frac{1}{|\mathcal{D}|}
\sum_{i\in\mathcal{D}}
\mathbf{1}\!\left[
\operatorname{parent}(\hat{v}_i)
=
\operatorname{parent}(v_i)
\right].
\end{equation}

\emph{Path accuracy} requires the entire root$\rightarrow$leaf path to match:
\begin{equation}
\mathrm{Acc}_{\text{path}}
=
\frac{1}{|\mathcal{D}|}
\sum_{i\in\mathcal{D}}
\mathbf{1}\!\left[
\operatorname{path}(\hat{v}_i)
=
\operatorname{path}(v_i)
\right].
\end{equation}

\subsection{Description Quality Metrics}
\label{sec:supp-desc-metrics}

We evaluate the quality of language descriptions paired with memory.

\begin{itemize}
  \item \textbf{Color Accuracy (Color Acc):} fraction of episodes where the described color attributes (e.g., “red mug”, “blue sofa”) match the ground-truth annotations.
  \item \textbf{Loc@parent:} fraction of episodes where the location phrase correctly identifies the parent container or anchor in the tree (e.g., “on the side table next to the green sofa”).
  \item \textbf{Loc@path:} stricter variant requiring the full root$\rightarrow$leaf path implied by the description to match the ground-truth path (scene, room/anchor, container, object).
\end{itemize}

These metrics are computed from human-annotated ground truth and the textual outputs aligned with the corresponding memory nodes.

\subsection{Instruction Quality and Error Analysis}
\label{sec:supp-error-metrics}

We separately analyze the quality of step-by-step instructions and the types of errors that occur, independent of raw success rates.

\subsubsection*{Category proportions}

Over all labeled errors (an episode may have multiple tags), let
$E_{\mathrm{P}},E_{\mathrm{R}},E_{\mathrm{M}}$ be counts of
\emph{Planning}, \emph{Reasoning}, and \emph{Perception/Memory} errors, respectively.
We report their proportions:
\begin{align}
\mathrm{Err}_{\mathrm{P}}
&=
\frac{E_{\mathrm{P}}}{E_{\mathrm{P}}+E_{\mathrm{R}}+E_{\mathrm{M}}}, \\
\mathrm{Err}_{\mathrm{R}}
&=
\frac{E_{\mathrm{R}}}{E_{\mathrm{P}}+E_{\mathrm{R}}+E_{\mathrm{M}}}, \\
\mathrm{Err}_{\mathrm{M}}
&=
\frac{E_{\mathrm{M}}}{E_{\mathrm{P}}+E_{\mathrm{R}}+E_{\mathrm{M}}}.
\end{align}

\subsubsection*{Subtype breakdown}

For each top-level type $X\in\{\mathrm{P},\mathrm{R},\mathrm{M}\}$ and subtype “sub” with count $E_{X,\text{sub}}$, we define:
\begin{align}
\mathrm{Err}_{X,\text{sub}\,|\,X}
&=
\frac{E_{X,\text{sub}}}{E_X},
\\
\mathrm{Err}_{X,\text{sub}}^{\text{global}}
&=
\frac{E_{X,\text{sub}}}{E_{\mathrm{P}}+E_{\mathrm{R}}+E_{\mathrm{M}}}.
\end{align}

The subtypes are:
\begin{itemize}
  \item \emph{Planning} — wrong goal/room, missed step, wrong order, inefficient detour.
  \item \emph{Reasoning} — spatial relation mistake, logical inconsistency, insufficient exploration.
  \item \emph{Perception/Memory} — hallucinated object/landmark, wrong recognition, mislocalization.
\end{itemize}

\section{Runtime Breakdown}
\label{sec:supp-runtime}

We report additional timing statistics for the SpatialMem pipeline, including end-to-end preprocessing time and the per-task testing-time information referenced in the main paper.

\paragraph{Offline preprocessing.}
SpatialMem requires an initial preprocessing stage to convert the egocentric RGB stream into a metric 3D memory. The full pipeline timing is as follows:

\begin{itemize}
  \item \textbf{Point-cloud generation and alignment:}  
  Approximately \textbf{30 minutes} for global pose estimation, point-cloud fusion, and gravity alignment.

  \item \textbf{3D bounding-box extraction and automatic annotation:}  
  Around \textbf{5 minutes} for lifting 2D detections/masks into 3D and generating preliminary object boxes.

  \item \textbf{Memory-tree construction and vector-database generation:}  
  Roughly \textbf{15 minutes} for building the hierarchical memory structure (anchors, objects, relations) and creating the associated retrieval index.
\end{itemize}

\paragraph{Task-level inference time.}
Testing-time performance for navigation, object retrieval, and description queries follows the values reported in the main paper. These measurements cover end-to-end inference on the constructed memory, including query parsing, geometric reasoning, and answer generation. Detailed data can also be found in table~\ref{size_and_time}.
